# Supplementary material for: 3D Molecular Generation via Virtual Dynamics
Source: arXiv:2302.05847 source file (2023-02-12)
Supplement: Supplementary file 1 [file appendix_target.tex]

\begin{figure}[ht]
\centering
\includegraphics[width=0.75\linewidth]{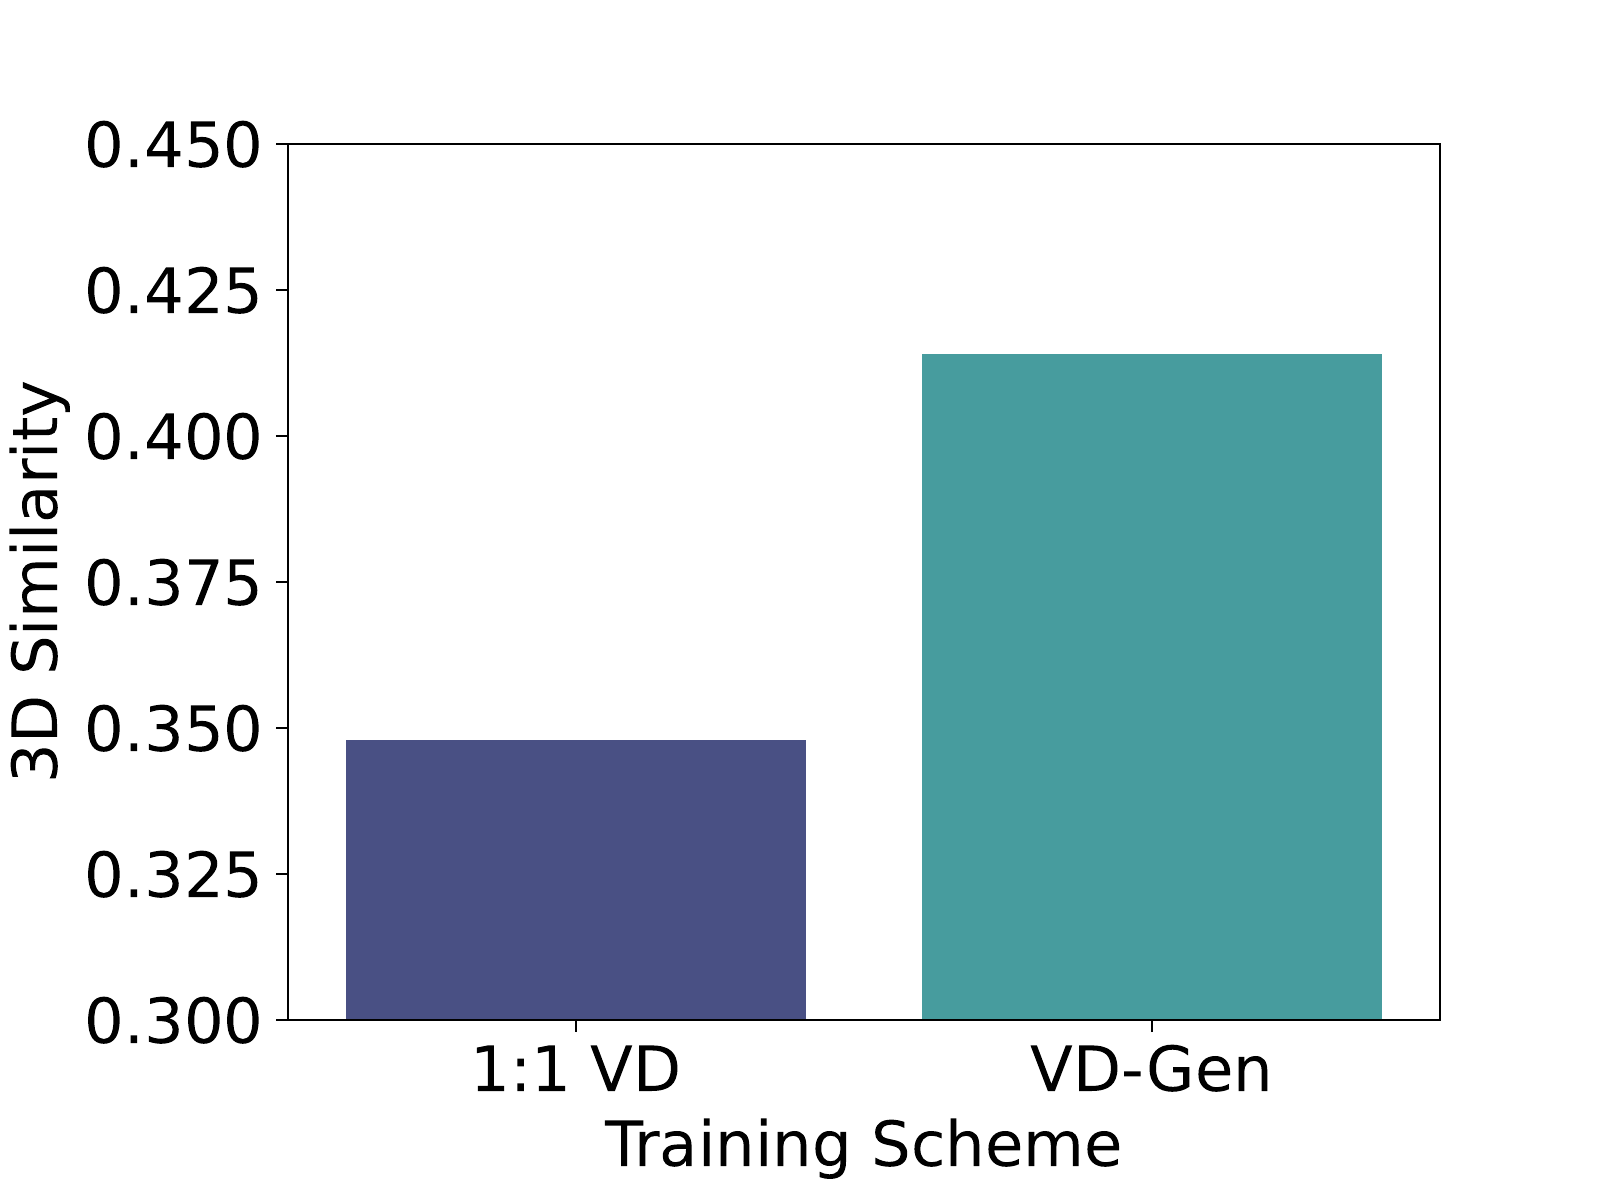}%
\caption{Comparison for different training frameworks. "1:1 VD" is our early attempt, which is directly based on \texttt{Virtual Dynamics}, with 1:1 particle-atom assignment, and without the 4 stages in \texttt{VD-Gen}. The result indicates the effectiveness of the proposed \texttt{VD-Gen} framework.} \label{fig:ablation_target}
\end{figure}%
